# Supplementary material for: Searching For Music Mixing Graphs: A Pruning Approach
Source: arXiv:2406.01049 source file (2024-08-06)
Supplement: Supplementary file 1 [file prune_process_appendix.tex]

\begin{figure*}
    \vspace{-3.5mm}
    \centering
    \includegraphics[width=2.08\columnwidth]{figures/pdf/appendix_prune_plot_real_appendix.pdf}
\caption{
Hello!
}
\label{fig:prune_process_appendix} 
\end{figure*}
